# Supplementary material for: Theoretical Analysis of Sparse Optimization with Reparameterization, Weight Decay, and Adaptive Learning Rate
Source: arXiv:2605.25134 source file (2026-05-29)
Supplement: Supplementary file 1 [file proof-convergence.tex]

\section{Proof of Convergence}

\begin{theorem}
    Assume that $f(\cdot)$ is $L$-Lipschitz and $M$-smooth, for $\eta_t = 1/\sqrt{T}$ and $\lambda = 1/T$. 
    Assume that $\x(t)$ is bounded by $\| \x(t) \| \leq C_x$.
    It holds that for \ReWA,
    \begin{equation*}
    \min_{t \in [T]} \| \x^{\frac{K-1}{2K}}(t) \odot \nabla f(\x(t))\| \leq T^{-1/4}.
\end{equation*}
\end{theorem}

\begin{proof}
We rewrite the iteration in \ReWA as
\begin{equation}
    w(t+1) = [(1-\lambda \eta_t) w^{1/K}(t) - \eta_t \nabla f(w(t))]^K. 
\end{equation}
We note that the power is element-wise. 
Therefore, we rewrite the iteration by Taylor expansion as
\begin{equation}
    \begin{split}
  &(1-\lambda \eta_t)^K w(t) \\
  -&\eta_t K  (1-\lambda \eta_t)^{K-1} w^{\frac{K-1}{K}}(t) \odot \nabla f(w(t))  \\
  +& \eta_t^2 \frac{K(K-1)}{2}  (1-\lambda \eta_t)^{K-2}  (\nabla f(w(t)))^2 \odot w^{\frac{K-2}{K}}(t) \\
  +& O(\eta_t^3).
\end{split}
\end{equation}
    
\end{proof}

We assume that $f(\cdot)$ is $L$-Lipschitz and $M$-smooth.

Then it holds that due to smoothness (the power is element-wise)
\begin{equation}
\begin{split}
    &f(w(t+1))\\
    \leq &f((1-\lambda \eta_t)^K w(t)) \\
    &- \nabla f^\top((1-\lambda \eta_t)^K w(t)) \eta_t K  (1-\lambda \eta_t)^{K-1} w^{\frac{K-1}{K}}(t) \odot \nabla f(w(t)) \\
    &+  \nabla f^\top((1-\lambda \eta_t)^K w(t)) \eta_t^2 \frac{K(K-1)}{2}  (1-\lambda \eta_t)^{K-2}  (\nabla f(w(t)))^2 \odot w^{\frac{K-2}{K}}(t) \\
    &+ M \| \eta_t K  (1-\lambda \eta_t)^{K-1} w^{\frac{K-1}{K}}(t) \odot \nabla f(w(t)) - \eta_t^2 \frac{K(K-1)}{2}  (1-\lambda \eta_t)^{K-2}  (\nabla f(w(t)))^2 \odot w^{\frac{K-2}{K}}(t)\|^2 \\
    &+ O(L \eta_t^3)
\end{split}
\end{equation}

Set $\eta_t = O(1/\sqrt{T})$ and $\lambda = 1/T$. 

For the first line, it holds that
\begin{equation}
    f((1-\lambda \eta_t)^K w(t)) - f(w(t)) \leq L ((1-\lambda \eta_t)^K - 1) \|w(t) \| \leq L C_w K \lambda \eta = O(1/T^{3/2}).  
\end{equation}

Similarly, 
\begin{equation}
    \nabla f((1-\lambda \eta_t)^K w(t)) - \nabla f(w(t)) \leq M C_w K \lambda \eta = O(1/T^{3/2}).  
\end{equation}

For the second line, it equals to
\begin{equation}
\begin{split}
   & \eta_t K  (1-\lambda \eta_t)^{K-1}  \nabla f^\top((1-\lambda \eta_t)^K w(t))  w^{\frac{K-1}{K}}(t) \odot \nabla f(w(t)) \\
    =& \eta_t K  (1-\lambda \eta_t)^{K-1} \nabla f^\top((w(t))  w^{\frac{K-1}{K}}(t) \odot \nabla f(w(t)) + O(1/T^{3/2})  \\
    = &  \eta_t K (1-\lambda \eta_t)^{K-1} \| w^{\frac{K-1}{2K}}(t) \odot \nabla f(w(t))\|^2 + O(1/T^{3/2})\\
\end{split}
\end{equation}

For the third line, it equals to
\begin{equation}
\begin{split}
    &\eta_t^2 \frac{K(K-1)}{2}  \nabla f^\top((1-\lambda \eta_t)^K w(t))  (1-\lambda \eta_t)^{K-2}  (\nabla f(w(t)))^2 \odot w^{\frac{K-2}{K}}(t) \\
    =& \eta_t^2 \frac{K(K-1)}{2}  (1-\lambda \eta_t)^{K-2}  \| (\nabla f(w(t)))^{3/2} \odot w^{\frac{K-2}{2K}}(t)\|^2+ O(1/T^{3/2}) \\
    \leq &  \eta_t^2 K^2 (1-\lambda \eta_t)^{K-2}  \| (\nabla f(w(t)))^{3/2} \odot w^{\frac{K-2}{2K}}(t)\|^2+ O(1/T^{3/2}) \\
\end{split}
\end{equation}

For the fourth line, it equals to (we omit some $\eta_t^3$ term)
\begin{equation}
\begin{split}
    & M \| \eta_t K  (1-\lambda \eta_t)^{K-1} w^{\frac{K-1}{K}}(t) \odot \nabla f(w(t))\|^2 \\
    = & M \eta_t^2 K^2  (1-\lambda \eta_t)^{2(K-1)} \|w^{\frac{K-1}{K}}(t) \odot \nabla f(w(t)) \|^2 \\
    \leq & M \eta_t^2 K^2  (1-\lambda \eta_t)^{K-2} \|w^{\frac{K-1}{K}}(t) \odot \nabla f(w(t)) \|^2 
\end{split}
\end{equation}

In summary, it holds that
\begin{equation}
    \begin{split}
    &f(w(t+1))\\
    \leq &f(w(t)) \\
    &- \eta_t K (1-\lambda \eta_t)^{K-1} \| w^{\frac{K-1}{2K}}(t) \odot \nabla f(w(t))\|^2 \\
    &+ \eta_t^2K^2 (1-\lambda \eta_t)^{K-2} (  \|w^{\frac{K-2}{2K}}(t) \odot (\nabla f(w(t)))^{3/2}\|^2 + M \|w^{\frac{K-1}{K}}(t) \odot \nabla f(w(t)) \|^2  ) \\
    &+ O(1/T^{3/2})
\end{split}
\end{equation}

Therefore, by letting $\eta_t \leq ...$, it holds that

\begin{equation}
    \begin{split}
    f(w(t+1))
    \leq f(w(t))- \frac{1}{2} \eta_t K (1-\lambda \eta_t)^{K-1} \| w^{\frac{K-1}{2K}}(t) \odot \nabla f(w(t))\|^2+ O(1/T^{3/2})
\end{split}
\end{equation}

Taking sum, and taking average, it holds that
\begin{equation*}
   \sum_t  \| w^{\frac{K-1}{2K}}(t) \odot \nabla f(w(t))\|^2 \leq C.
\end{equation*}
Therefore, 
\begin{equation*}
    \min_t \| w^{\frac{K-1}{2K}}(t) \odot \nabla f(w(t))\| \leq T^{-1/4}.
\end{equation*}

Therefore, it is equivalent to minimizing the loss
\begin{equation*}
    f(w^{\frac{3K-1}{2K}})
\end{equation*}
